# Supplementary material for: Accurate dust temperature determination in a $z = 7.13$ galaxy
Source: arXiv:2108.13479 source file (2021-09-27)
Supplement: Supplementary file 4 [file journals.tex]

% Astrophysics and Space Science
              % Planetary and Space Science
