# Supplementary material for: Accurate dust temperature determination in a $z = 7.13$ galaxy
Source: arXiv:2108.13479 source file (2021-09-27)
Supplement: Supplementary file 5 [file package.tex]

\usepackage{txfonts}
\usepackage[T1]{fontenc}
\usepackage{ae,aecompl}

\usepackage{graphicx}

% to avoid conflict let amsmath redefine some stuff
\let\iiint=\relax
\let\iiiint=\relax
\let\idotsint=\relax
\let\iint=\relax
\usepackage{amsmath}
\usepackage{amsfonts}
\usepackage{amssymb}

\usepackage{xcolor}

\usepackage{breakcites}
\usepackage{hyperref}
\usepackage{footnote}

\usepackage{comment}

\usepackage{xfrac}
